# Supplementary material for: V-SlowFast Network for Efficient Visual Sound Separation
Source: arXiv:2109.08867 source file (2021-09-21)
Supplement: Supplementary file 1 [file vis_sep_supp_MUSIC21.pdf]

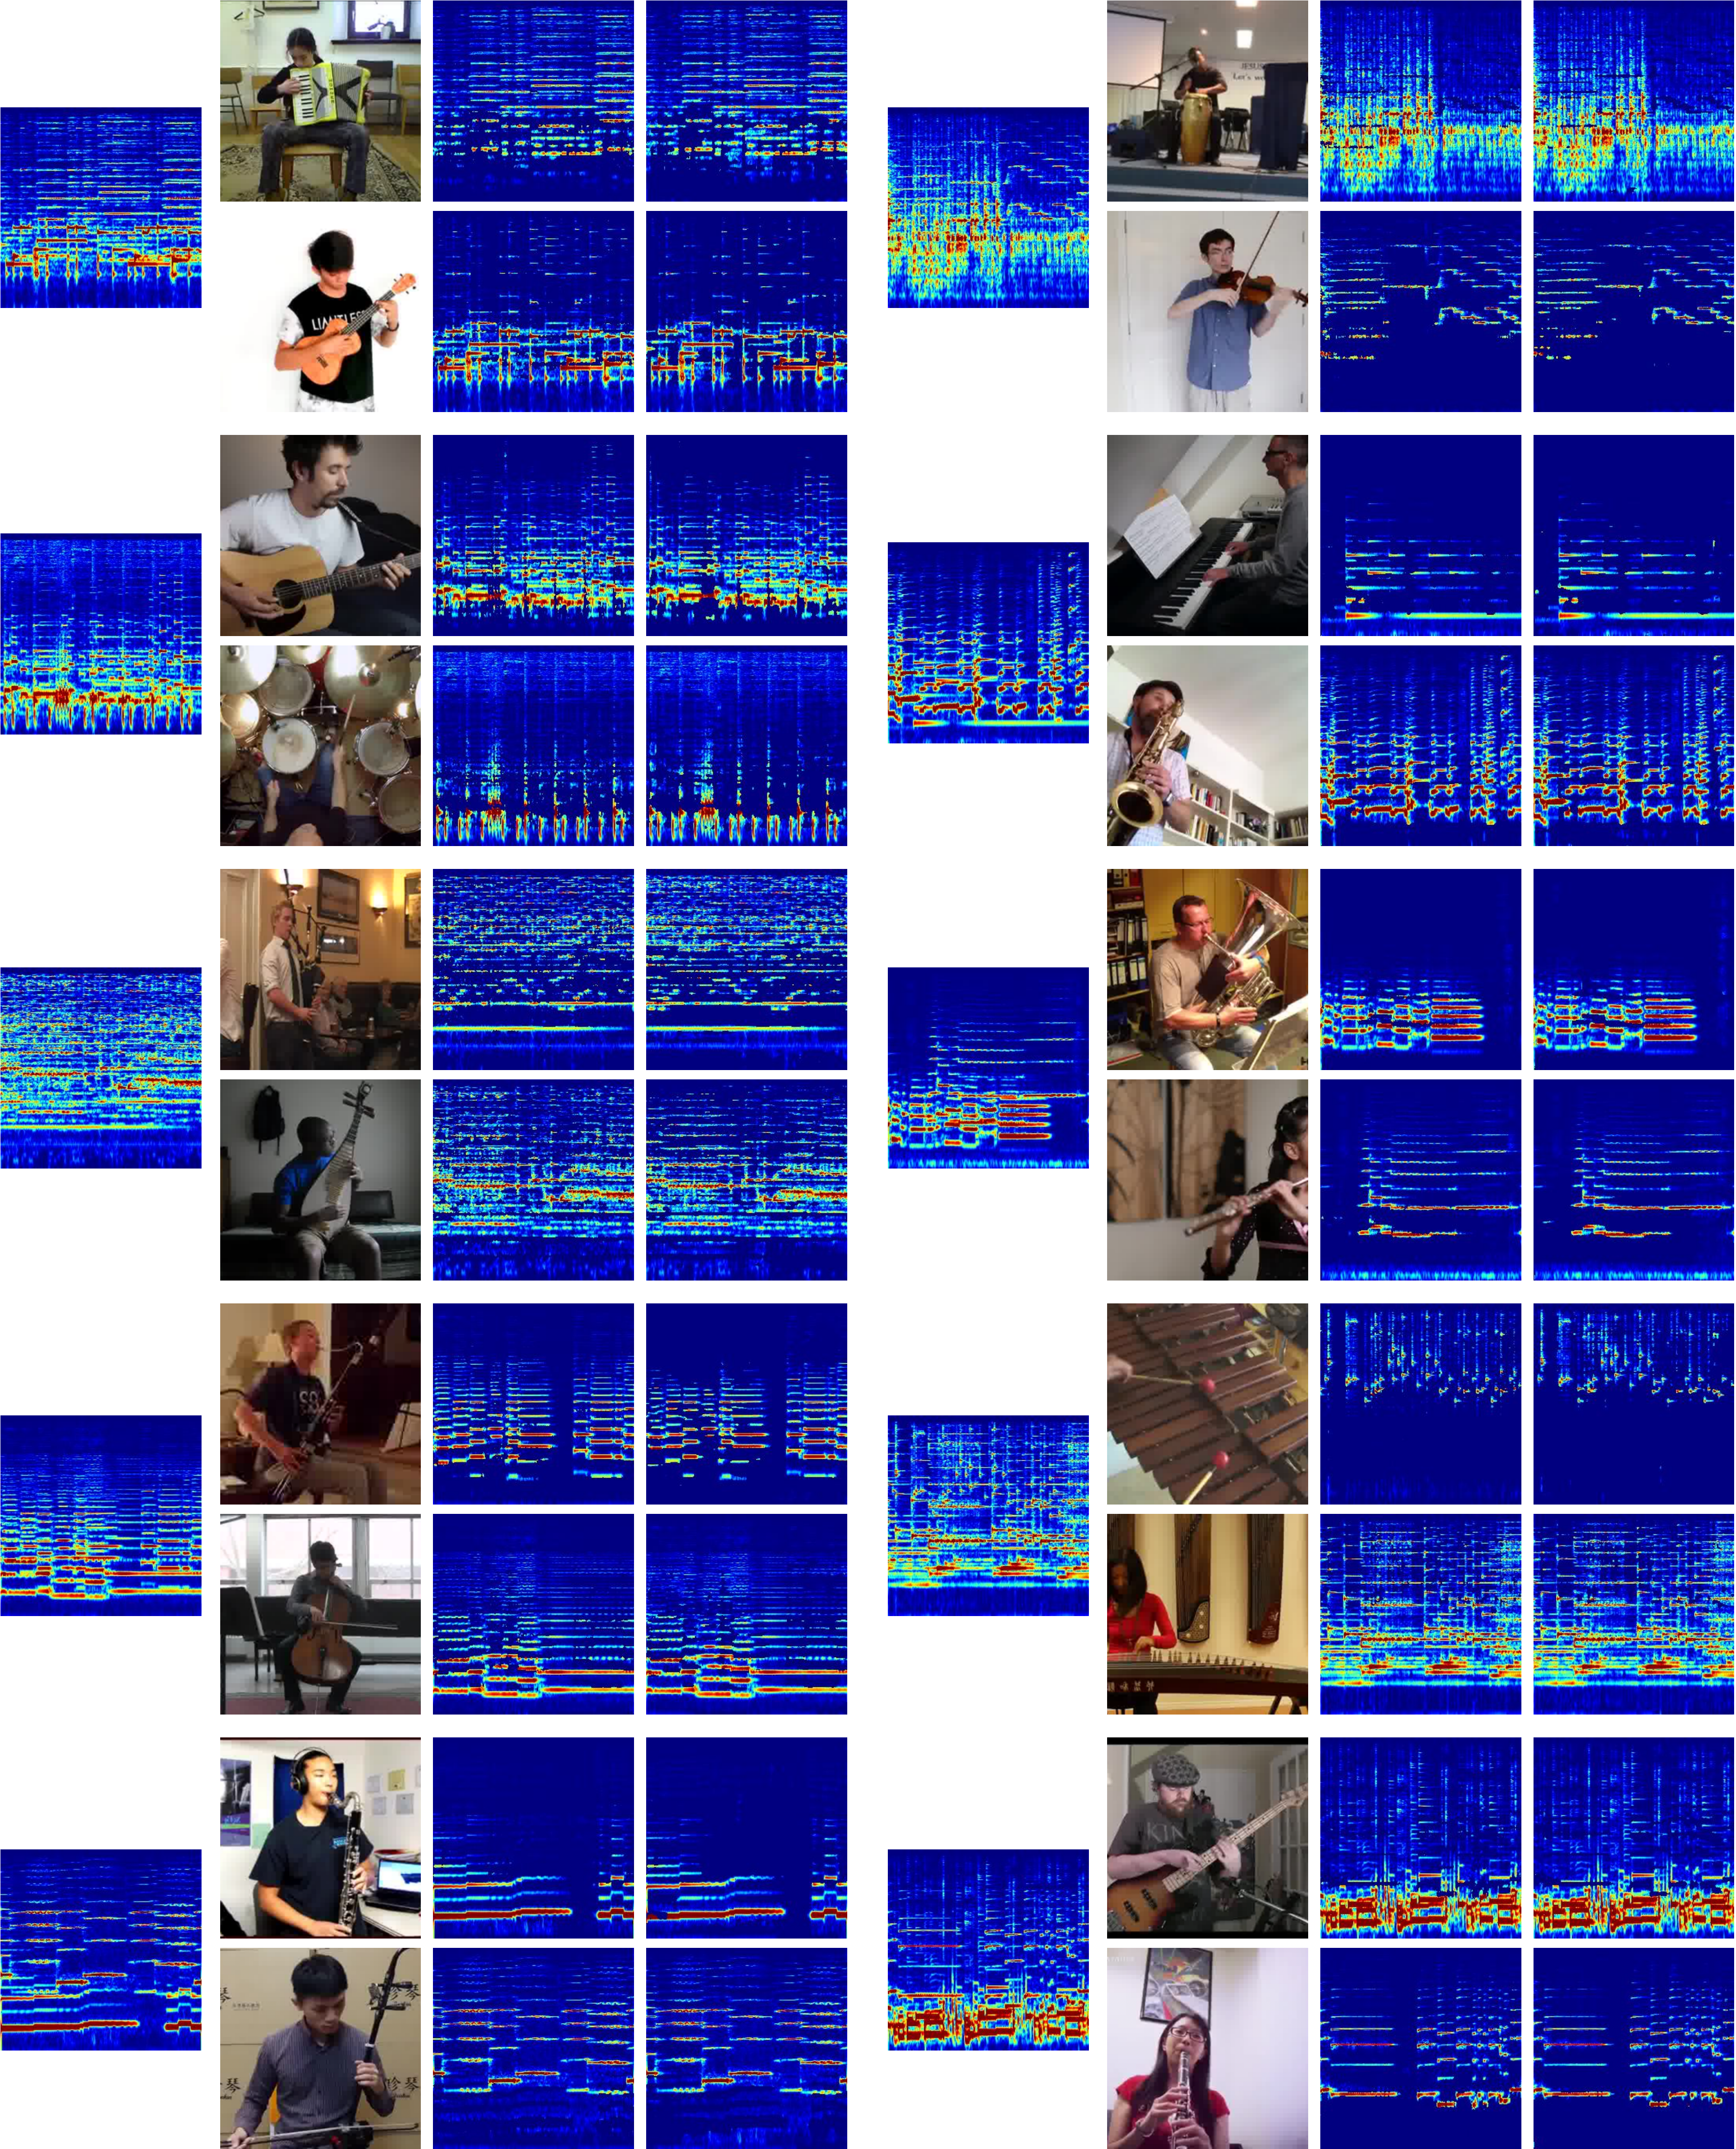

Mixture      Frame      GT      V-SlowFast      Mixture      Frame      GT      V-SlowFast
